# Supplementary material for: Tuning metal-insulator transitions in epitaxial V$_2$O$_3$ thin films
Source: arXiv:1801.07075 source file (2018-04-03)
Supplement: Supplementary file 1 [file V2O3_Supplementary.pdf]

# Tuning metal-insulator transitions in epitaxial $V_2O_3$ thin films

## Supplementary material

Einar B. Thorsteinsson,[1] Seyedmohammad Shayestehaminzadeh,[2] and Unnar B. Arnalds[1]
[1]*Science Institute, University of Iceland, Dunhaga 3, 107 Reykjavik, Iceland*
[2]*Technovation Centre, AGC Glass Europe, Rue Louis Blériot 12, BE-6041 Gosselies, Belgium*

## I. EXPERIMENTAL INFORMATION

### A. Sample growth

The $V_2O_3$ films were grown in a custom-built magnetron sputtering chamber[1]. The target to substrate distance was 17 cm. Prior to growth the base pressure was in all cases below $2 \times 10^{-6}$ Pa. Argon gas of 99.999% purity mixed with oxygen gas of purity 99.999% was used for the reactive sputtering process. The argon flow rate into the chamber was kept constant at 20 sccm and the $O_2$ flow rate varied within 1.4 sccm and 2.0 sccm for this study. The total pressure during sputtering was maintained at 0.4 Pa using a throttle valve. Figure S1 shows the dependence of the chamber pressure with $O_2$ flow setting. The oxygen pressure component increases linearly above the initial argon pressure with increasing $O_2$ flow. Flow settings below 1 sccm were not detectable with the capacitance manometer. A Vanadium target of 99.5% purity and 3" diameter (75 mm) was used in a planar magnetron configuration. The films were grown on one side polished single crystalline $Al_2O_3$[0001] substrates from CrysTec gmbh (1 mm thick and size $1 \times 1$ cm$^2$). Prior to growth all substrates were cleaned in acetone, isopropanol and methanol, each for 5 minutes in ultrasonic bath, and subsequently rinsed in DI water and dried with nitrogen gas. Before deposition the samples were baked inside the sputtering chamber at a temperature of 650°C for at least 25 minutes and then another 20 minutes at the growth temperature. At the growth temperature, prior to introducing argon and oxygen into the chamber, the base pressure was in all cases at or below $1 \times 10^{-5}$ Pa. After growth the heater in the sputtering chamber was turned off and the film allowed to cool down *in situ* to room temperature.

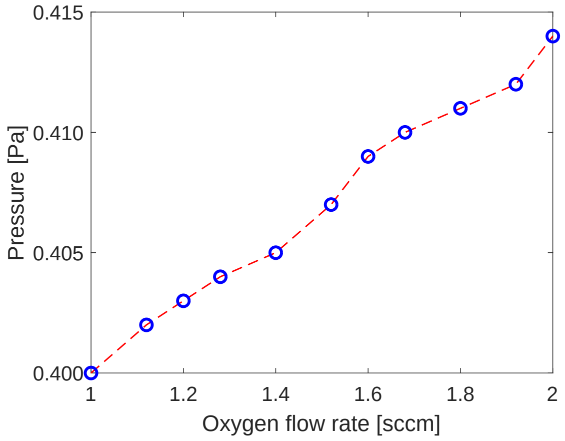


FIG. S1: Graph showing the total pressure in the deposition chamber for different $O_2$ flow settings. Initially, argon was introduced into the chamber at a flow setting of 20 sccm. Subsequently, the chamber throttle valve was adjusted to obtain a chamber pressure of 0.400 Pa as measured by a capacitance manometer. After this, the $O_2$ flow setting was increased and the chamber pressure recorded.

### B. Materials characterization

The X-ray diffraction and reflectivity curves were recorded using a Panalytical X'Pert PRO diffractometer mounted with a hybrid monochromator/mirror on the incident side and a 0.27 parallel plate collimator on the diffracted side.

A line focus was used with a beam width of approximately 1 mm. Reciprocal space mapping was performed using a triple axis setup with an analyzer crystal with a 12" acceptance angle. Rocking curve scans of the film peaks were also performed with the triple axis setup. The film thickness and surface roughness was quantified by x-ray reflectivity and simulations using the X'PERT Reflectivity program. The surface morphology of the films was investigated by atomic force microscopy using a Park XE-100 instrument in both contact as well as non-contact mode. The resistance of the films was measured in the temperature range 10 K to 300 K using a Cryogenic CFMS system. The resistance was measured using a Keithley 2400 Sourcemeter connected to a Keithley 7001 switch system with a 7012-S $4 \times 10$ matrix card. The maximum resistance measurable by the experimental setup was limited to $\sim 5 \times 10^9$ Ω. After deposition, 100 nm thick gold electrodes were deposited by e-beam evaporation along the edges of the films using a shadow mask to provide contact to the films.

## II. RECIPROCAL SPACE MAPS

The reciprocal space maps were recorded with a 0D point detector and a triple axis analyzer crystal (12″ acceptance angle) on the diffracted side, while a hybrid 2-bounce monochromator was on the incidence side. The $Al_2O_3$ (1 0 -1 10) peak of the substrate was used as an internal reference and used to calibrate the position of the x-ray machine. The calibrated positional value used was calculated from the $a$ and $c$ lattice parameters taken from the certificate of the NIST standard reference material 1976b.

For the sake of higher resolution scans in a reasonable amount of time, the whole region was not scanned in a single scan, instead it was broken up into different smaller regions. Firstly, a small high resolution scan around the substrates $Al_2O_3$ (1 0 -1 10) peak. Secondly, a larger scan around the $V_2O_3$ (1 0 -1 10) peak position. Thirdly, a series of 13 small high resolution scans of the fully strained portion of the $V_2O_3$ located at the $Q_x$ value of the substrate. The scan times were respectively 2, 14 and 5 hours, for a total of around 21 hours per sample.

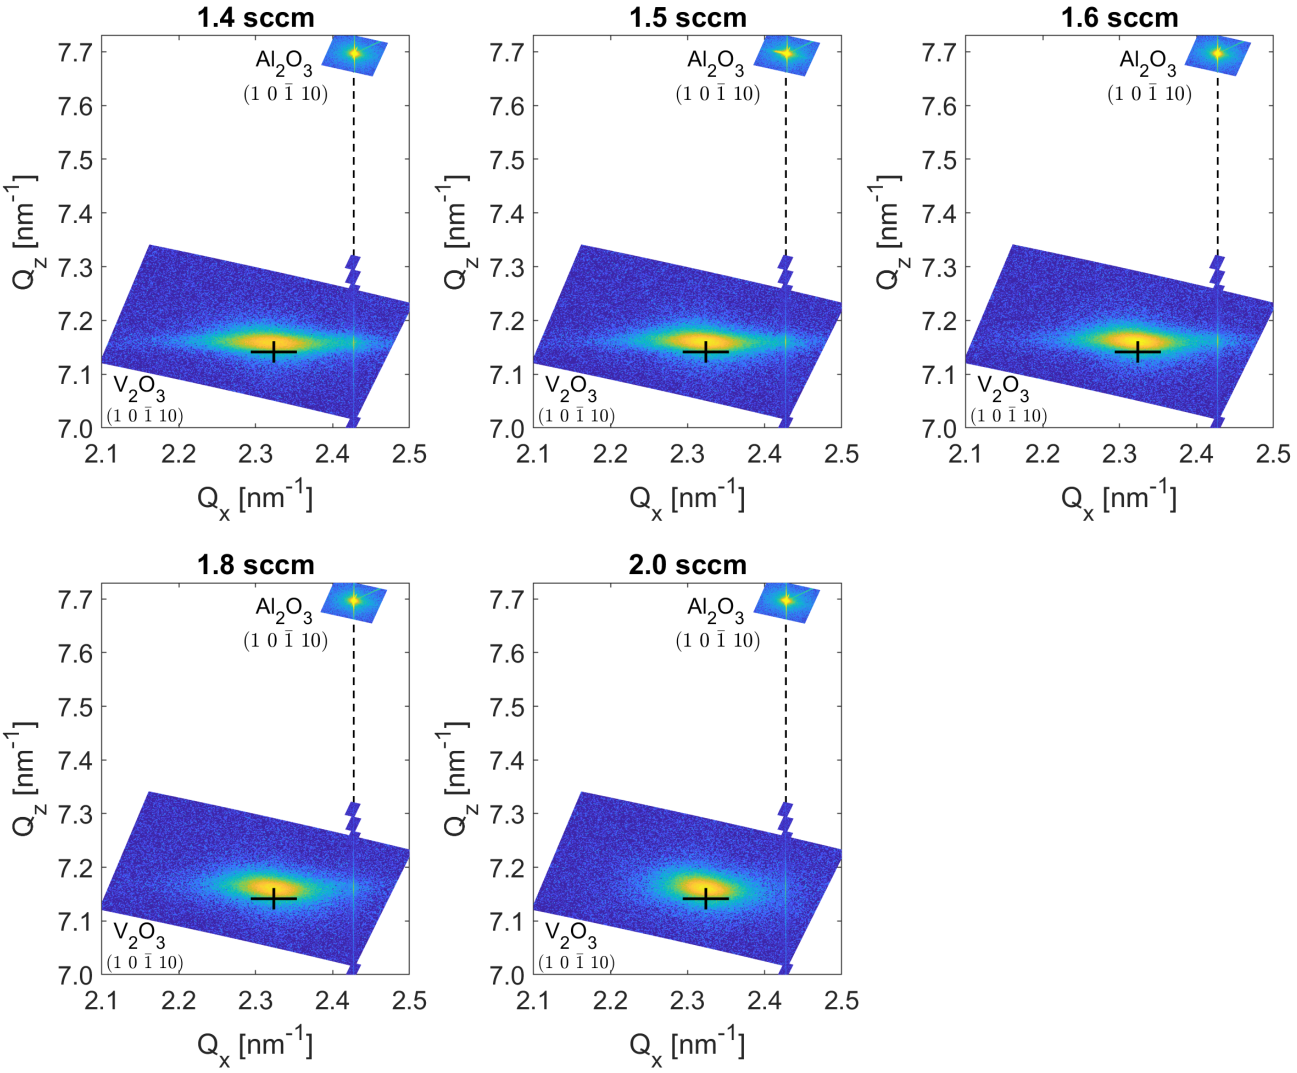


FIG. S2: Compilation of reciprocal space maps recorded for films deposited under different $O_2$ conditions around the (1 0 -1 10) peak. The crosses illustrate the location of the peak for bulk $V_2O_3$. For the graphs the $\log_{10}$(Intensity) is plotted using the Matlab parula colormap with the color axis limited to the highest intensity value recorded for the $V_2O_3$ peaks. The intensity of the $Al_2O_3$ substrate peak is therefore not depicted correctly.

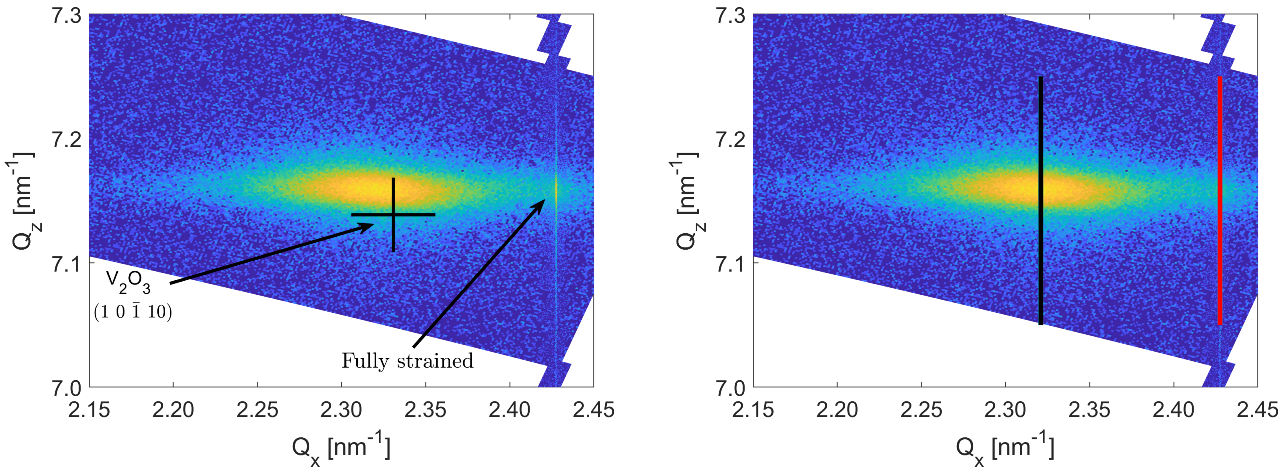


FIG. S3: A focused view of the RSM peaks of the 1.4 sccm sample. On the right are the black and red lines indicating the area that are sampled for figure S4.

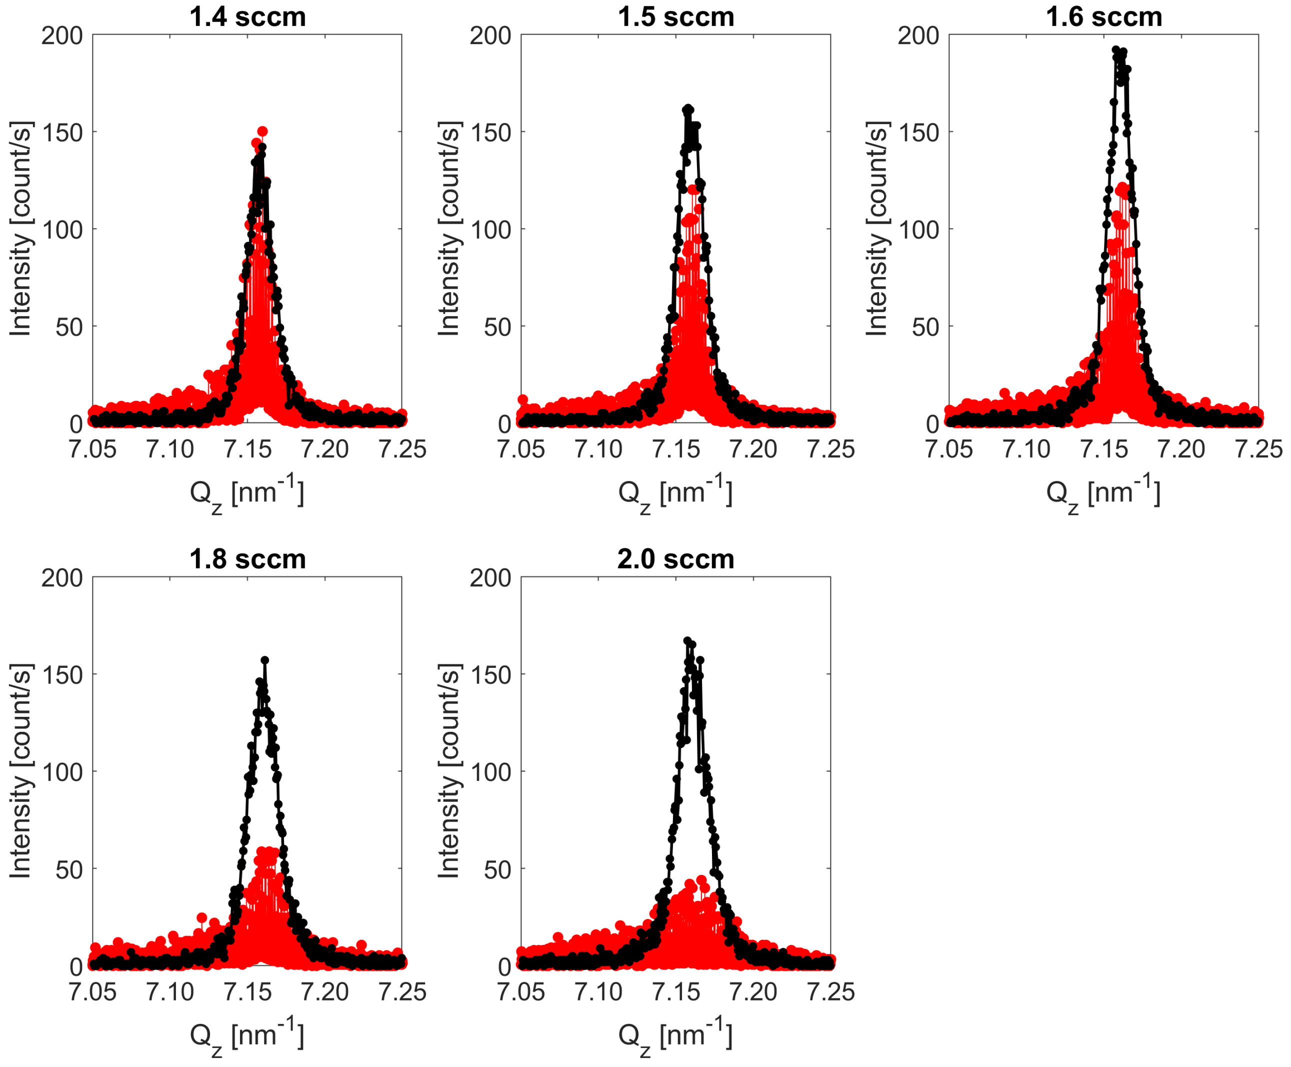


FIG. S4: The intensity of the relaxed and fully strained peak as a function of $Q_z$. Black is taken from the large relaxed peak, while red is taken from the thin fully strained lattice matched peak, as indicated by figure S3.

## III. LATERAL CORRELATION LENGTH AND MOSAICITY

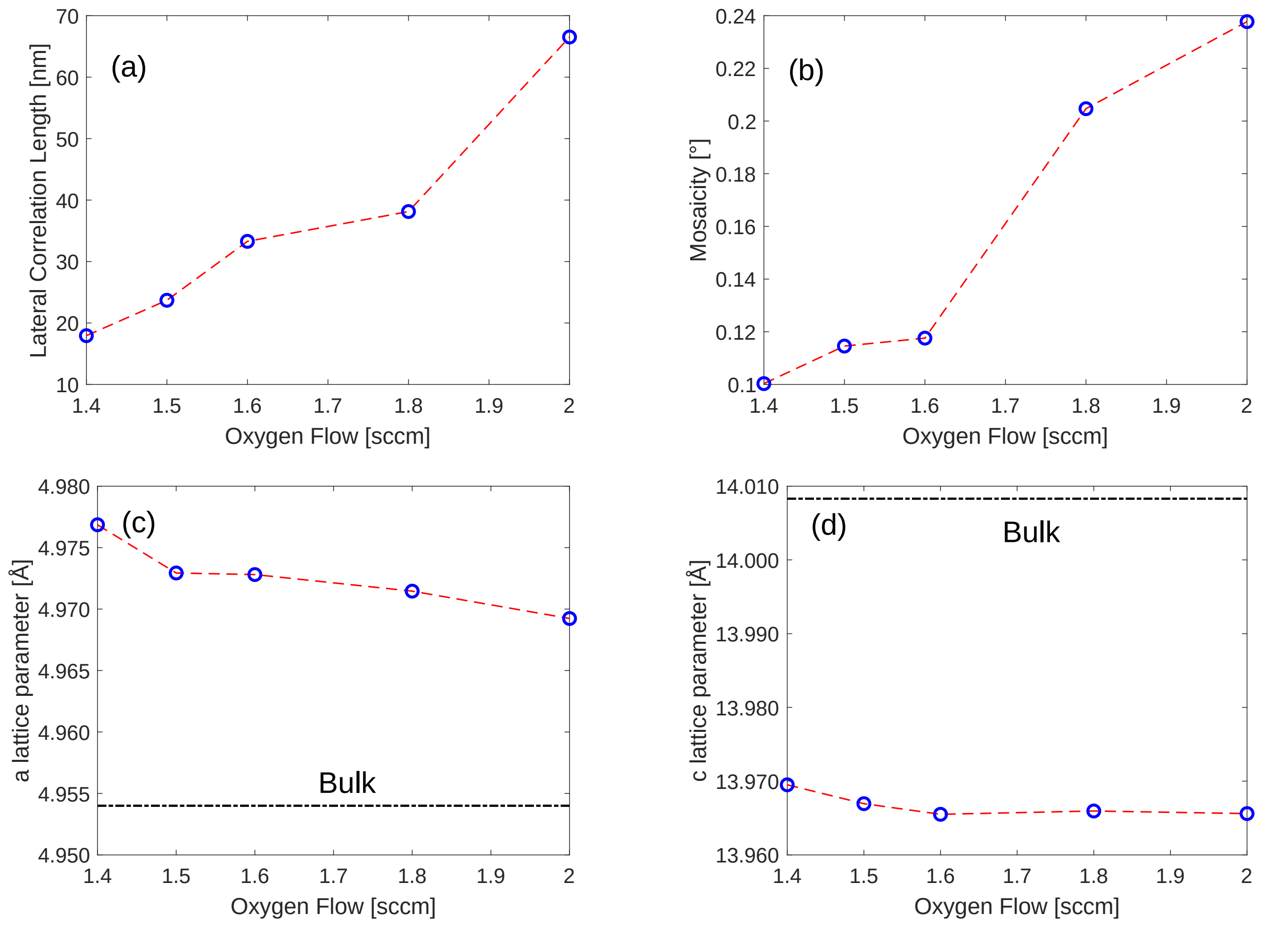


FIG. S5: (a) Lateral correlation length, (b) mosaicity, (c) a lattice parameter and (d) c lattice parameter extracted from the (1 0 -1 10) $V_2O_3$ peaks shown in figure S2.

## IV. POWER SERIES

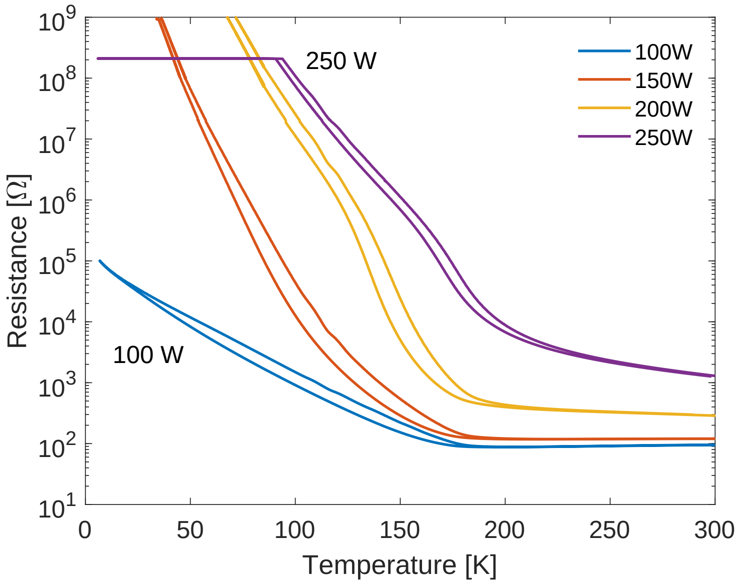


FIG. S6: Resistance as a function of temperature for samples grown under different sputtering powers. All samples were grown with the same oxygen flow rate of 1.6 sccm at 0.4 Pa pressure and 485°C growth temperature. The saturation in the 250W sample is a result of the range not switching properly in the Keithley 2400 sourcemeter. It can be noted that the 200W, 1.6 sccm film has values very similar to the 150W, 1.4 sccm film in the main paper.


[1] U. B. Arnalds, J. S. Agustsson, A. S. Ingason, A. K. Eriksson, K. B. Gylfason, J. T. Gudmundsson, and S. Olafsson, Review of Scientific Instruments **78**, 103901 (2007).
